# Supplementary material for: Suppression of multiphoton resonances in driven quantum systems via pulse shape optimization
Source: arXiv:1703.04165 ancillary file (2017-08-03)
Supplement: Supplementary file 1 [file SM.pdf]

# SUPPLEMENTARY MATERIAL – Suppression of multiphoton resonances in driven quantum systems via pulse shape optimization

Denis Gagnon,[1,2,*] François Fillion-Gourdeau,[1,2] Joey Dumont,[1] Catherine Lefebvre,[1,2] and Steve MacLean[1,2,†]

[1]*Université du Québec, INRS–Énergie, Matériaux et Télécommunications, Varennes, Québec, Canada, J3X 1S2*

[2]*Institute for Quantum Computing, University of Waterloo, Waterloo, Ontario, Canada, N2L 3G1*

(Dated: August 3, 2017)

* denis.gagnon@uwaterloo.ca

† steve.maclean@uwaterloo.ca

## I. STRONGLY DRIVEN TWO-LEVEL SYSTEMS

In this work, we use the following two-level Hamiltonian as a starting point for Floquet calculations (Eq. 1 in the Letter):

$$H(t) = -\frac{\varepsilon(t)}{2}\sigma_z - \frac{\Delta}{2}\sigma_x. \tag{1}$$

This particular choice of representation is usual in the description of ac-driven superconducting quantum circuits [1, 2]. We will now show how other Hamiltonians can be mapped onto Eq. (1) using unitary transformations, as described in Ref. [1]. Unitary transformations do not affect the transition probabilities calculated via Floquet theory. In addition, the transition probability is unchanged by a change of sign in the coefficients of Eq. (1) as also described in Ref. [1].

*a. Atoms and molecules in laser fields, semiconductor superlattices.* The Hamiltonian (1), with a field coupling in diagonal terms (proportional to $\sigma_z$), can be transformed to the typical Hamiltonian used to describe light matter interaction in atoms and molecules, where the field coupling appears in off-diagonal terms (proportional to $\sigma_y$). This can be achieved using the following unitary transformation [1]:

$$H'(t) = \exp\left[-i\frac{\pi}{4}\sigma_y\right] H(t) \exp\left[i\frac{\pi}{4}\sigma_y\right] \tag{2}$$

which leads to

$$H'(t) = -\frac{\Delta}{2}\sigma_z - \frac{\varepsilon(t)}{2}\sigma_x. \tag{3}$$

This Hamiltonian is frequently used for the description of the optical response of atoms and molecules (see e.g Grifoni and Hänggi [3, p. 244]). In this physical setting, $\varepsilon(t)$ is proportional to the dipole moment of the atomic system and the amplitude of the applied field, while $\Delta$ is the energy splitting term due to tunnelling [3]. Without further modification, Eq. (1) also describes the tunneling between quantum wells in semiconductor nanostructures (see e.g. Platero and Aguado [4, p. 10]).

Let us now show how to obtain the differential equations describing Rabi oscillations starting from the Hamiltonian (3). This development is presented in Ref. [3, p. 246]. Suppose the following ac excitation, describing a linearly polarized applied field:

$$\varepsilon(t) = \varepsilon_0 \cos\omega t. \tag{4}$$

Substituting Eq. (4) in (3) yields

$$H'(t) = -\frac{1}{2}\begin{pmatrix} \Delta & \varepsilon_0\cos\omega t \\ \varepsilon_0\cos\omega t & -\Delta \end{pmatrix}. \tag{5}$$

Now, suppose the following Ansatz for the wavefunction:

$$\psi(t) = c_1(t)\exp\left[i\frac{\Delta t}{2}\right]\begin{pmatrix}1\\0\end{pmatrix} + c_2(t)\exp\left[-i\frac{\Delta t}{2}\right]\begin{pmatrix}0\\1\end{pmatrix}. \tag{6}$$

Substituting this Ansatz in the Schrödinger equation with the Hamiltonian (3) yields, after basic manipulations:

$$\dot{c_1}(t) = \frac{i\varepsilon_0}{4}\Big(\exp\left[i(\omega-\Delta)t\right] + \exp\left[-i(\omega+\Delta)t\right]\Big)c_2(t) \tag{7a}$$

$$\dot{c_2}(t) = \frac{i\varepsilon_0}{4}\Big(\exp\left[-i(\omega-\Delta)t\right] + \exp\left[i(\omega+\Delta)t\right]\Big)c_1(t). \tag{7b}$$

These two rate equations describe the population of the lower and upper excited level, respectively. They can be further simplified by making the usual rotating-wave approximation, i.e. by assuming that the ac driving frequency $\omega$ is close to the energy detuning $\Delta$, which allows one to neglect fast oscillating terms (terms with $(\omega+\Delta)t$ dependence). This approximation yields the usual differential equations for Rabi oscillations in quantum optics:

$$\dot{c_1}(t) = \frac{i\varepsilon_0}{4}\exp\left[i\delta t\right]c_2(t) \tag{8a}$$

$$\dot{c_2}(t) = \frac{i\varepsilon_0}{4}\exp\left[-i\delta t\right]c_2(t). \tag{8b}$$

with $\delta \equiv \omega - \Delta$, and where the factor $\frac{\varepsilon_0}{4}$ is usually called *Rabi frequency.* These differential equations are equivalent to those found in Boyd, for instance [**?** , p. 285].

*b. Dirac materials.* The results of this Letter may also be applied to Dirac materials such as graphene [5]. Consider Dirac fermions (for instance, in a graphene mono-layer) in the presence of a linearly polarized laser field, which is uniform in space and normally incident to the 2D-material plane. The fermion dynamics are governed by the following low energy Hamiltonian

$$H_\xi(t,\mathbf{p}) = \xi v_F \boldsymbol{\sigma}\cdot[\mathbf{p} + e\mathbf{A}(t)], \tag{9}$$

where $\xi = \pm 1$ is the valley pseudospin index, $v_F$ is the Fermi velocity of the Dirac material, $\boldsymbol{\sigma} = (\sigma_x, \sigma_y)$ is a vector of Pauli matrices representing the sublattice pseudospin, $\mathbf{p}$ is the

fermion momentum around the $K^\xi$ points (for instance, graphene has two inequivalent $K$ points) and $-e < 0$ is the electron charge. Consider that the applied field is given by the following vector potential: $\mathbf{A}(t) = [A_x(t), 0]$. A change of representation of the Dirac matrices can be performed via a unitary transformation to obtain a Hamiltonian closer to the canonical form of a strongly driven two-level atom [6]:

$$H'_\xi(t, \mathbf{p}) = U_r^\dagger H_\xi(t, \mathbf{p}) U_r \tag{10}$$

where

$$U_r \equiv \exp\left[-i\sigma_x \frac{\pi}{4}\right] \exp\left[-i\sigma_y \frac{\pi}{4}\right]. \tag{11}$$

Combining this transformation with the following change of variables

$$\Delta \equiv -2\xi v_F p_y, \tag{12a}$$

$$\varepsilon(t) \equiv -2\xi v_F [p_x + eA_x(t)], \tag{12b}$$

leads to

$$H'_\xi(t, \mathbf{p}) = -\frac{\varepsilon(t)}{2}\sigma_z - \frac{\Delta}{2}\sigma_x. \tag{13}$$

This is the same functional form as the superconducting qubit Hamiltonian considered in the Letter, Eq. (1). The limits of validity of Eq. (13) for the description of real-world laser-irradiated graphene are detailed in Refs. [6, 7].

## II. OPTIMIZATION CALCULATIONS

This supplementary section contains technical details about the optimization calculations presented in the accompanying Letter. A certain familiarity with metaheuristics is assumed: we refer the interested reader to Ref. [8] for more details.

*a. Generalized island model.* Optimization runs are executed on a highly parallel supercomputer using the MPI implementation of the PAGMO optimization library [9]. The number of MPI islands is set to 48, as each node on the supercomputer has 24 processors and 2 nodes are used for each optimization run. In fact, only 47 islands are used since a processor is used to manage communication between nodes. The 47 islands form an "archipelago" which is connected using a simple ring topology. This means that information on optimal solutions is transferred between an island and only 2 neighboring islands. The efficiency of

the combination of DE + ring topology comes from a good balance between intensification (exploiting the neighborhood of good solutions) and diversification (migrating to new search neighborhoods). In actuality, as detailed in Ref. [10], DE does not seem to benefit from a quick spread of information when compared with other metaheuristics.

All solutions on all islands are initialized at random, i.e. no prior knowledge of "good solutions" is used in the optimization runs presented in this Letter.

*b. Choice of decision variables and bounds.* In this Letter, we consider odd periodic excitations which are represented by Fourier series of the form

$$g(t) = \sum_{n=1}^{\infty} b_n \sin n\omega t. \tag{14}$$

A monochromatic excitation, for example, corresponds to $b_n = 0$ for all $n$ except $b_1 = 1$. A triangle wave corresponds to a series representation with alternating signs, that is

$$b_n = \frac{(-1)^{(n-1)/2}}{n^2}, \qquad n = 1, 3, 5... \tag{15}$$

with $b_{2n} = 0$. The normalization of the triangle wave Fourier series is chosen such that the amplitude of the fundamental is equal to 1. The goal of using only odd periodic excitations, with alternating signs and odd order Fourier coefficients ($X_n = b_{2n-1}$) is to fall between the behavior of a sine wave and that of the triangle wave, in other words to have excitations which have a node at $T/2$. This choice is motivated by the fact that the optimization routine is based on an eigenvalue solver for the calculation of Floquet transition probabilities, and that the solver sometimes fails to converge because it encounters ill-conditioned matrices constructed from the Floquet Hamiltonian. We have found that odd periodic excitations with odd order Fourier coefficients minimize the failure rate of the eigenvalue solver, thereby enabling the optimization to proceed smoothly without wasting computational resources.

Additionally, we enforce alternating signs and use the following arbitrary bounds on optimization variables in all calculations presented in the letter.

$$\max(|X_n|) = \begin{cases} 1, & n = 1 \\ \dfrac{2}{2n-1}, & n > 1 \end{cases}, \tag{16}$$

$$\min(|X_n|) = \begin{cases} 0.66, & n = 1 \\ 0, & n > 1 \end{cases}. \tag{17}$$

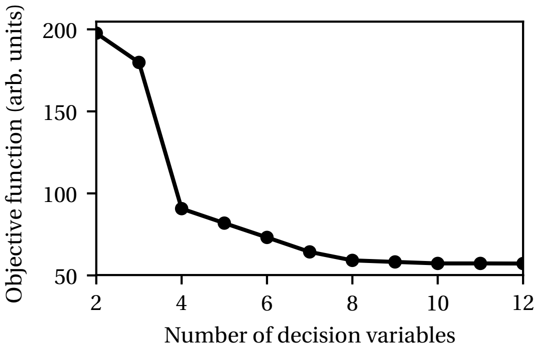


Figure A1. Best found solution as a function of the number of optimization variables (Fourier harmonics) used in DE. Each point corresponds to 20 generations and 47 parallel islands each containing a population of size 10.

Again, this choice is made in order for the optimization runs to proceed smoothly without failed eigenvalue decompositions caused by ill-conditioned matrices.

*c. Choice of the number decision variables.* We have run a set of optimization calculations similar to that found in Fig. 2, but with different sizes of $\vec{X}$, to show that using a high number of Fourier harmonics resulted in a stronger resonance suppression, equivalent to finding solutions with lower objective functions. The result of this set of optimization calculations is shown in Fig. A1. Every point on the plot corresponds to the same number of objective function evaluations, in other words to the same computational cost. The objective function gain is only marginal when increasing the number of Fourier harmonics over 10, which is partly due to the upper bound set on the optimization variables, Eq. (16). For this reason, we set the number of optimization variables to 10 in DE calculations.

*d. Best found solution.* The Fourier coefficients of the best solution found (shown in Fig. 2 of the Letter) are detailed in Table A1. For reference, the upper bound of the magnitude of every decision variable is shown in the Table. Only two decision variables ($X_3$ and $X_4$) hit their respective upper bound, whereas the variable $X_1$ hits the lower optimization bound.

[1] S. Shevchenko, S. Ashhab, and F. Nori, Phys. Rep. **492**, 1 (2010).

[2] H. Z. Jooya, K. Reihani, and S.-I. Chu, Sci. Rep. **6**, 37544 (2016).

| $n$ | $X_n(b_{2n-1})$ | $\max(\lvert X_n \rvert)$ |
|---|---|---|
| 1 | 0.660 | 1.000 |
| 2 | -0.518 | 0.667 |
| 3 | 0.400 | 0.400 |
| 4 | -0.285 | 0.286 |
| 5 | 0.2019 | 0.222 |
| 6 | -0.144 | 0.182 |
| 7 | 0.105 | 0.154 |
| 8 | -0.093 | 0.133 |
| 9 | 0.090 | 0.118 |
| 10 | -0.089 | 0.105 |

Table A1. Fourier coefficients found via DE, corresponding to the result shown in Fig. 2. The upper bound of the magnitude of every optimization variable is also shown for reference.


[3] M. Grifoni and P. Hänggi, Phys. Rep. **304**, 229 (1998).

[4] G. Platero and R. Aguado, *Phys. Rep.*, Vol. 395 (2004) pp. 1–157.

[5] S. Das Sarma, S. Adam, E. H. Hwang, and E. Rossi, Rev. Mod. Phys. **83**, 407 (2011).

[6] F. Fillion-Gourdeau, D. Gagnon, C. Lefebvre, and S. MacLean, Phys. Rev. B **94**, 125423 (2016).

[7] D. Gagnon, F. Fillion-Gourdeau, J. Dumont, C. Lefebvre, and S. MacLean, J. Phys. Condens. Matter **29**, 035501 (2017).

[8] E. Talbi, *Metaheuristics: From Design to Implementation* (Wiley, 2009).

[9] D. Izzo, in *Proceedings of the Fifth International Conference on Astrodynamics Tools and Techniques, ICATT* (2012).

[10] M. Rucinski, D. Izzo, and F. Biscani, Parallel Computing **36**, 555 (2010).
